# Supplementary material for: Ultra Fast Deep Lane Detection with Hybrid Anchor Driven Ordinal Classification
Source: arXiv:2206.07389 source file (2022-06-15)
Supplement: Supplementary file 1 [file llamas_supp.tex]

\begin{table}[h]
    \centering
    \caption{Comparison on the LLAMAS dataset.}
    \label{tab_llamas}
    \begin{tabular}{lcccc}
        \toprule
    Method              & F1    & Precision & Recall & FPS \\
    \midrule
    PolyLaneNet         & 88.40 & 88.87     & 87.93  & 115 \\
    LaneATT(ResNet-18)  & 93.46 & 96.92     & 90.24  & 250 \\
    LaneATT(ResNet-34)  & 93.74 & 96.79     & 90.88  & 171 \\
    LaneATT(ResNet-122) & 93.54 & 96.82     & 90.47  & 26  \\
    UFLDv2(ResNet-18)   & 94.58 & 95.29     & 93.88  & 285 \\
    UFLDv2(ResNet-34)   & 94.95 & 95.75     & 94.17  & 156  \\
    \bottomrule
    \end{tabular}
    \end{table}
